# Supplementary material for: Automated Discovery of Branching Rules with Optimal Complexity for the Maximum Independent Set Problem
Source: arXiv:2412.07685 source file (2024-12-10)
Supplement: Supplementary file 1 [file ex_supplement.tex]

% SIAM Supplemental File Template
\documentclass[review,supplement,onefignum,onetabnum]{siamart190516}

\input{ex_shared}

\externaldocument{ex_article}

% Optional PDF information
\ifpdf
\hypersetup{
  pdftitle={Supplementary Materials},
  pdfauthor={}
}
\fi

\begin{document}

\maketitle

\bibliographystyle{siamplain}
\bibliography{references}

\end{document}
